# Supplementary material for: Variational Option Discovery Algorithms
Source: arXiv:1807.10299 source file (2018-07-26)
Supplement: Supplementary file 2 [file appendix_toddler.tex]

\section{Extended Discussion for Toddler Results} \label{appendix-toddler}

For the learning curve reported in Fig. \ref{baby-curve}, we used a variant of VALOR which used observations as direct inputs to the decoder instead of $k$-step transitions. This improved the learning speed somewhat. We observed a similar effect in experiments in the Hand environment: using states instead of state differences as decoder inputs resulted in faster learning. This seems to stem from the choice of representation for states in these environments, which is predominantly based on joint angles with finite range.
